# Supplementary material for: Nuclear cusps and singularities in the non-additive kinetic potential bi-functional from analytical inversion
Source: arXiv:2207.04160 source file (2022-10-10)
Supplement: Supplementary file 1 [file Supp_info_vNAD.pdf]

Supporting Information:

Nuclear cusps and singularities in the  
non-additive kinetic potential bi-functional  
from analytical inversion

Mojdeh Banafsheh,<sup>\*,†</sup> Tomasz A. Wesolowski,<sup>\*,‡</sup> Tim Gould,<sup>\*,¶</sup> Leeor Kronik,<sup>\*,§</sup>  
and David A. Strubbe<sup>\*,†</sup>

<sup>†</sup>*Department of Physics, University of California, Merced, Merced, CA 95343*

<sup>‡</sup>*Département de Chimie Physique 30, Université de Genève, Quai Ernest-Ansermet,  
CH-1211 Genève 4, Switzerland*

<sup>¶</sup>*Queensland Micro- and Nanotechnology Centre, Griffith University, Nathan, QLD 4111,  
Australia*

<sup>§</sup>*Department of Department of Molecular Chemistry and Materials Science, Weizmann  
Institute of Science, Weizmann Institute of Science, Rehovoth 76100, Israel*

E-mail: mbanafsheh@ucmerced.edu; tomasz.wesolowski@unige.ch; t.gould@griffith.edu.au;  
leeor.kronik@weizmann.ac.il; dstrubbe@ucmerced.edu

# 1 Introduction

Here we explain the choice of different numerical parameters in DARSEC for the calculations in the paper, and demonstrate the precision and convergence. All plots shown are for the He-He diatomic system, with nuclei at  $(0, 0, \pm 3)$  Bohr.

## 2 Stencil for Gradient and Laplacian

DARSEC uses the finite-difference method for gradient and Laplacian calculations. The user can choose an even number between 2 and 20 for the number of points  $s$  in the finite-difference stencil. In the code  $s = 12$  is suggested as an appropriate choice. In Fig. S1,  $v^{\text{NAD/INV}}$  is shown calculated with different stencils (for the SCF run as well as for the analytic inversion, Eq. (9)). Values  $s \leq 10$  give deviations from the converged smooth behavior at the edges of the plateau, so we must use  $s \geq 12$  (Fig. S2). To choose a reliable stencil, we finally compared  $s = 12$  with  $s = 20$  at the region where the densities overlap. As shown in Fig. S4, the difference between these two choices is negligible except smaller differences at a distance around 15 Bohr from the system's center, which is not relevant for our study. The potentials from  $s = 12$  and  $s = 20$  at this region are shown in detail in this region in Fig. S5, where the Laplacian is more sensitive to the choice of the stencil (Fig. S3). Seeing that the code's general recommendation is sufficient, we choose  $s = 12$  for all further calculations.

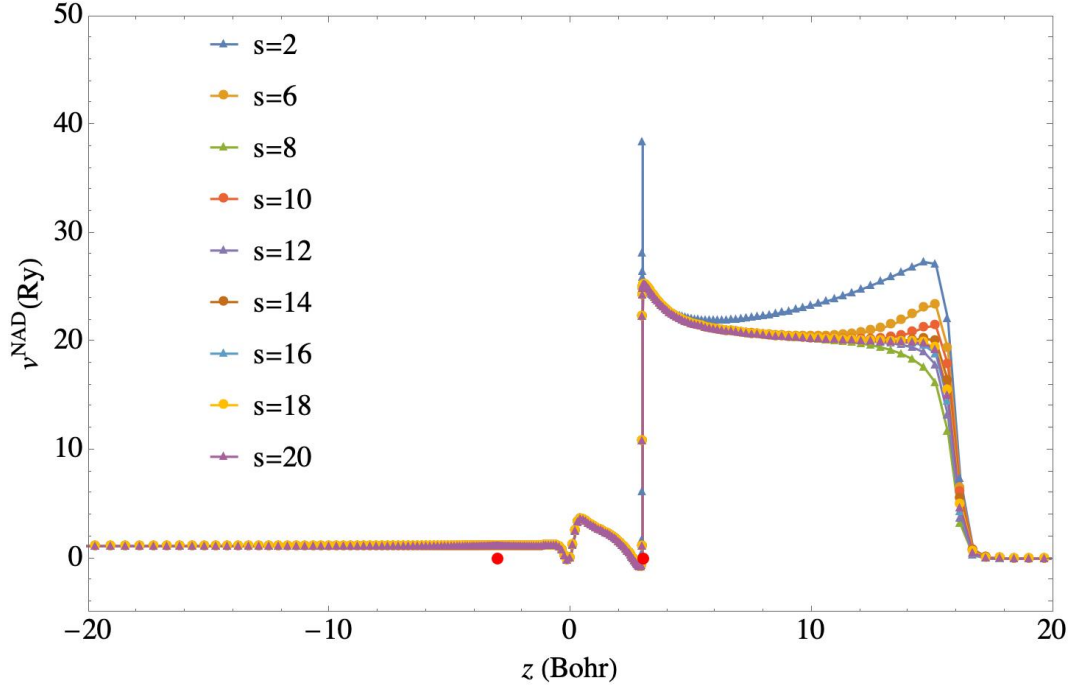

Figure S1: Comparison of  $v^{\text{NAD/INV}}$  calculated with different stencil sizes  $s$  for finite differences. Red dots indicate the  $z$  coordinates of the nuclei at  $\pm 3$  Bohr.

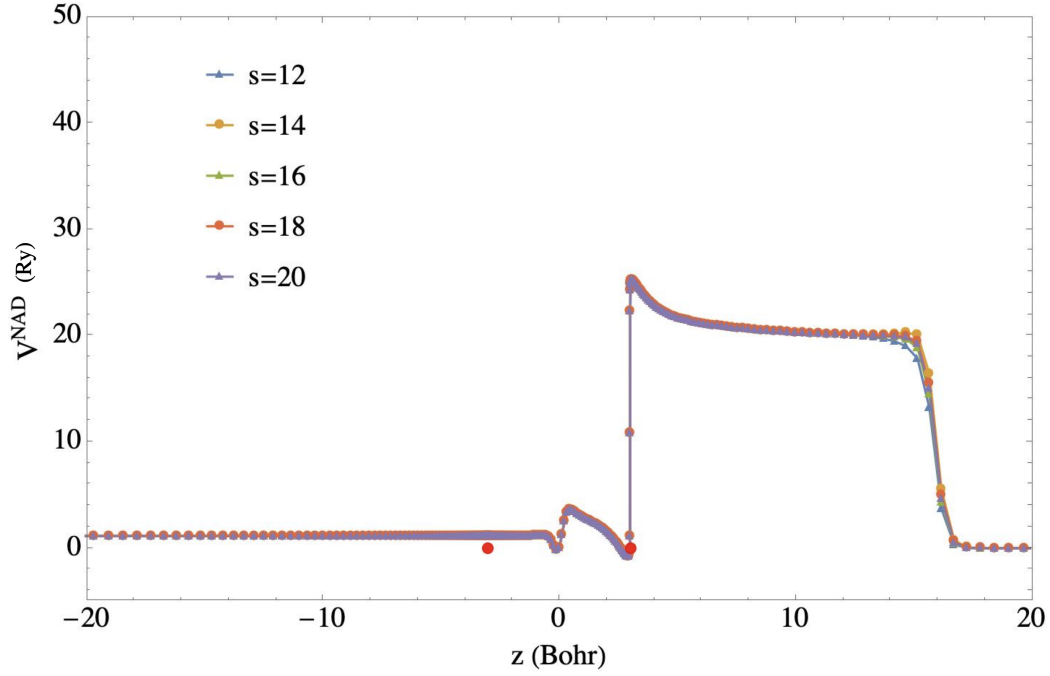

Figure S2: Comparison of  $v^{\text{NAD/INV}}$  as in Fig. S1, focusing on  $s \geq 12$ , showing smoother curves at the edges of the potential plateau.

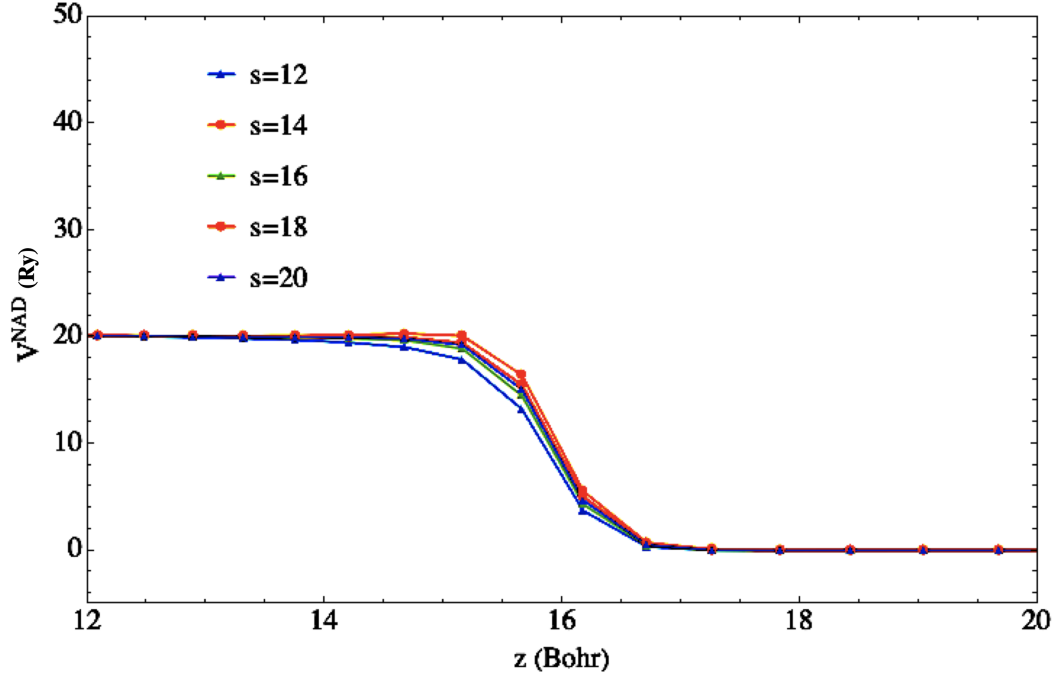

Figure S3: Comparison of  $v^{\text{NAD/INV}}$  as in Fig. S1, focusing on the right edge of the plateau. With the choice of  $s \geq 12$ , the curves are smooth and only show slight variation around 15 Bohr.

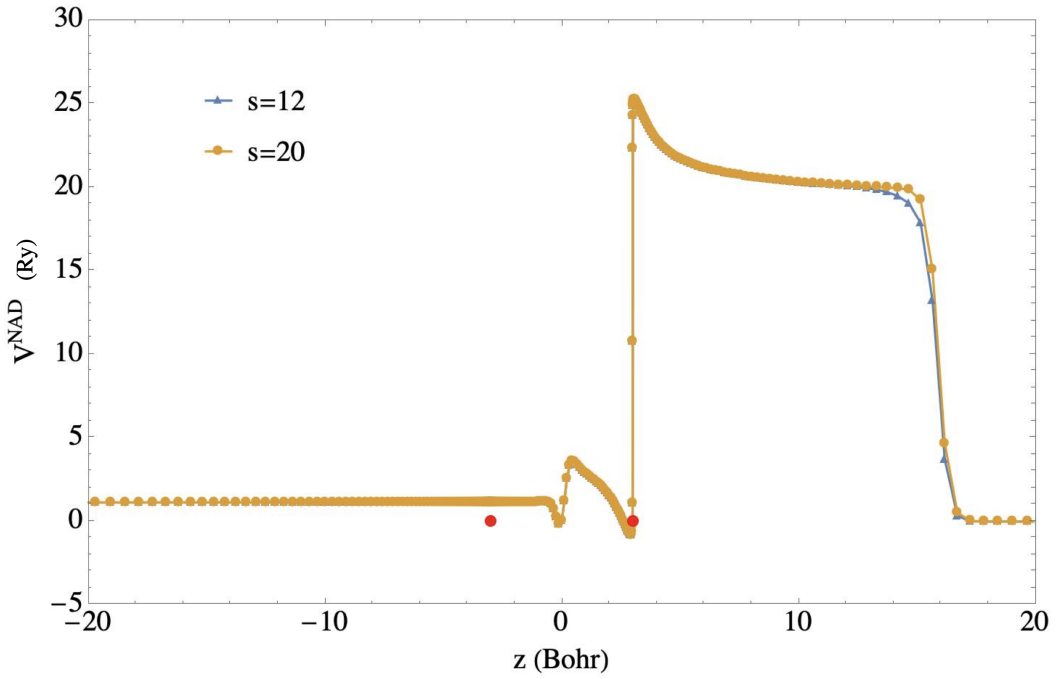

Figure S4: Comparison of  $v^{\text{NAD/INV}}$  as in Fig. S1, focusing on  $s = 12$  and  $s = 20$ , which show visible difference only around  $z = 15$  Bohr.

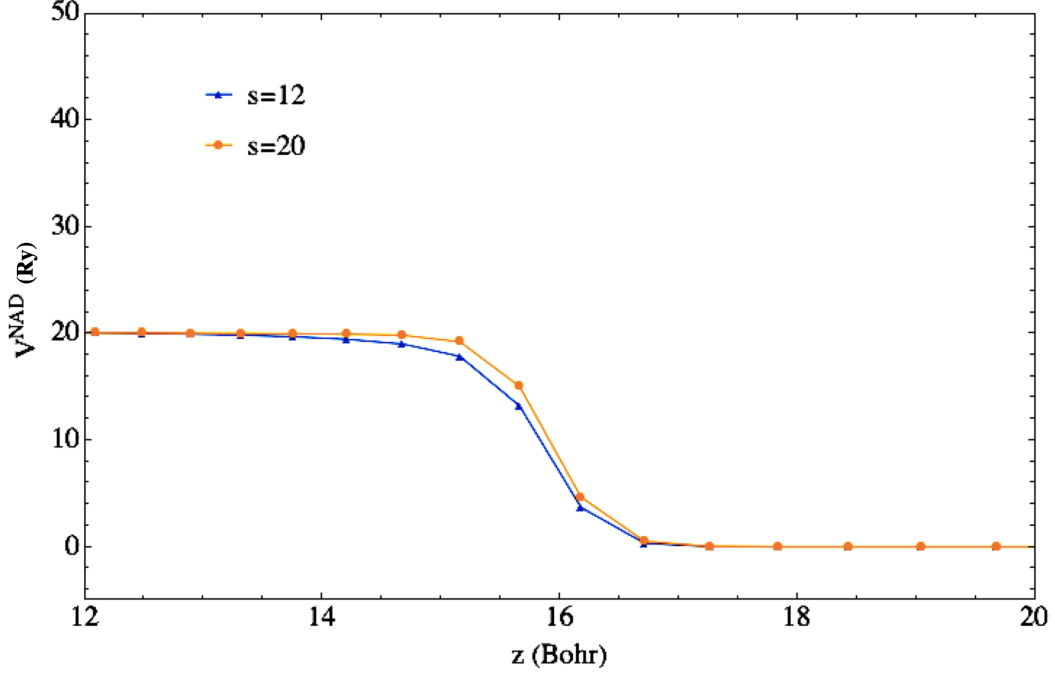

Figure S5: Comparison of  $v^{\text{NAD/INV}}$  as in Fig. S1, focusing on  $s = 12$  and  $s = 20$  at the right edge of the plateau. The maximum difference at  $z = 15$  Bohr is still small, and the density is very small in this region anyway so the differences have little impact.

### 3 Correction to possible division by zero

DARSEC doesn't provide the values on the  $z$ -axis since the Laplacian formulation is singular there. The diatomic systems we study in this work have only occupied states with  $m = 0$ , the angular momentum quantum number, and thus the density is nonzero on the  $z$ -axis. However, the density does tend to zero at long distance from the nuclei. When  $\rho \rightarrow 0$ , the denominator of the analytic inversion in Eq. (9) is singular which could cause numerical divergences. We made sure that such effects are not occurring in our calculations by adding a value  $\delta$  into the denominators to guarantee a nonzero minimum value, and observing its influence:

$$v^{\text{NAD/INV}}[\rho_B, \rho_{\text{tot}}](\mathbf{r}) = \frac{1}{2} \frac{\nabla^2 \sqrt{\rho_B(\mathbf{r})}}{\sqrt{\rho_B(\mathbf{r})} + \delta} - \frac{1}{2} \frac{\nabla^2 \sqrt{\rho_1(\mathbf{r})}}{\sqrt{\rho_1(\mathbf{r})} + \delta} \quad (1)$$

From Fig. S6, S7, and S8, we see that if the correction  $\delta \leq 1 \times 10^{-10} \sqrt{e/\text{Bohr}}$ , there is no perceptible difference to  $v^{\text{NAD/INV}}$ , except at extremely long range where the calculations are not reliable for other reasons. In Fig. S9, we see that with no correction applied to the calculations (case 0 in the graph), the results remain the same. As a result, we do not use  $\delta$  in our calculations.

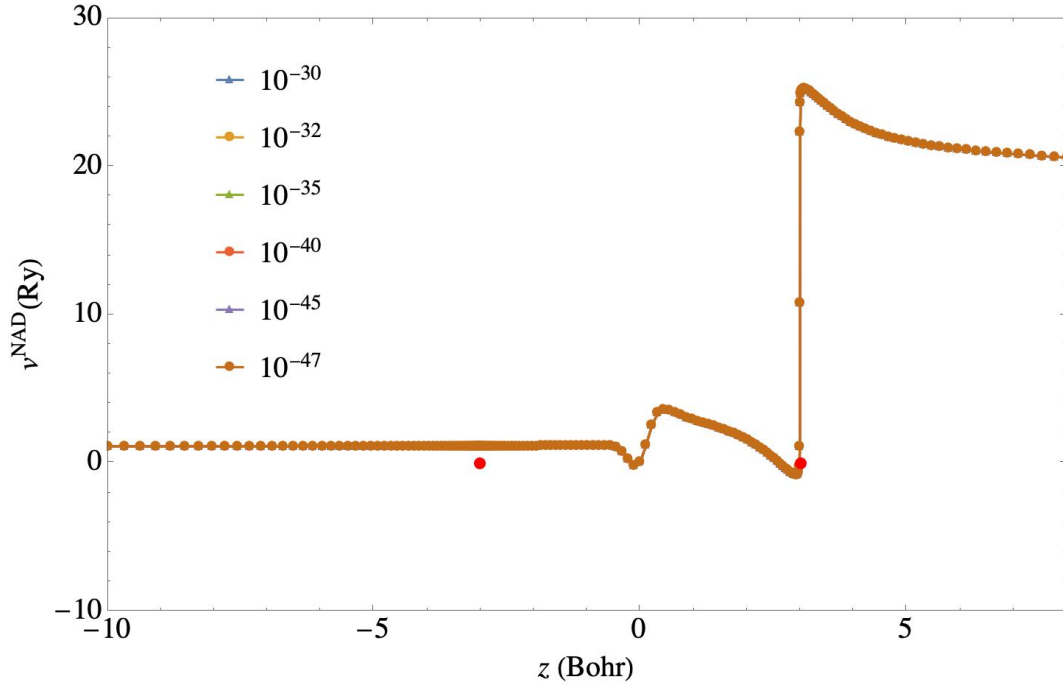

Figure S6: Comparison of  $v^{\text{NAD/INV}}$  with  $\delta$  term (in  $\sqrt{e/\text{Bohr}}$ ) added to denominators to avoid singularities. There is no perceptible difference for  $\delta$  varying from  $10^{-10}$  to  $10^{-47} \sqrt{e/\text{Bohr}}$ . Red dots indicate the  $z$  coordinates of the nuclei at  $\pm 3$  Bohr.

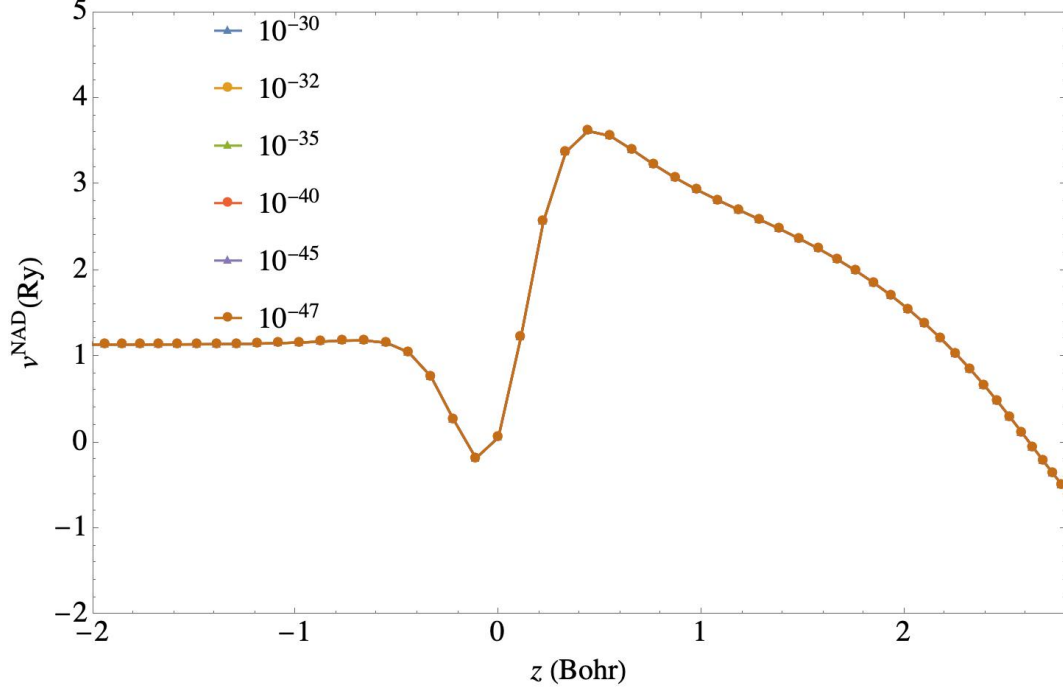

Figure S7: Detail of Fig. S6 in the region where the overlap of the densities tends to be maximum, for different values of  $\delta$  (in  $\sqrt{e/\text{Bohr}}$ ) added to denominators.

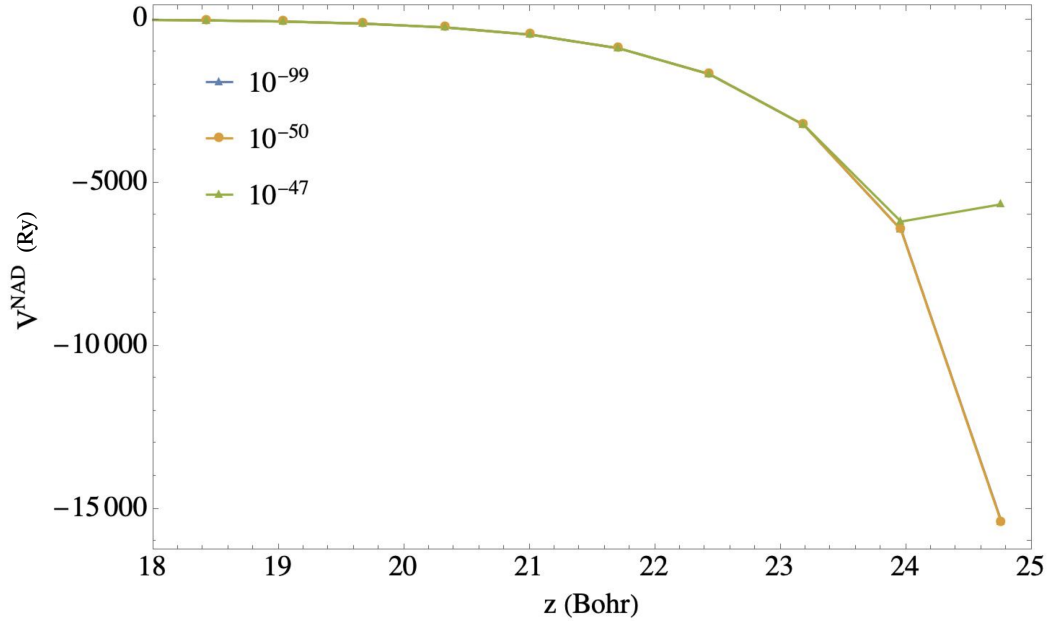

Figure S8: Detail of Fig. S6 far from the nuclei, for different values of  $\delta$  (in  $\sqrt{e/\text{Bohr}}$ ) added to denominators. With very small values of  $\delta$ , the potential may vary at large distances, outside our region of interest. The large negative values here are not meaningful anyway and are due to other numerical difficulties in this region.

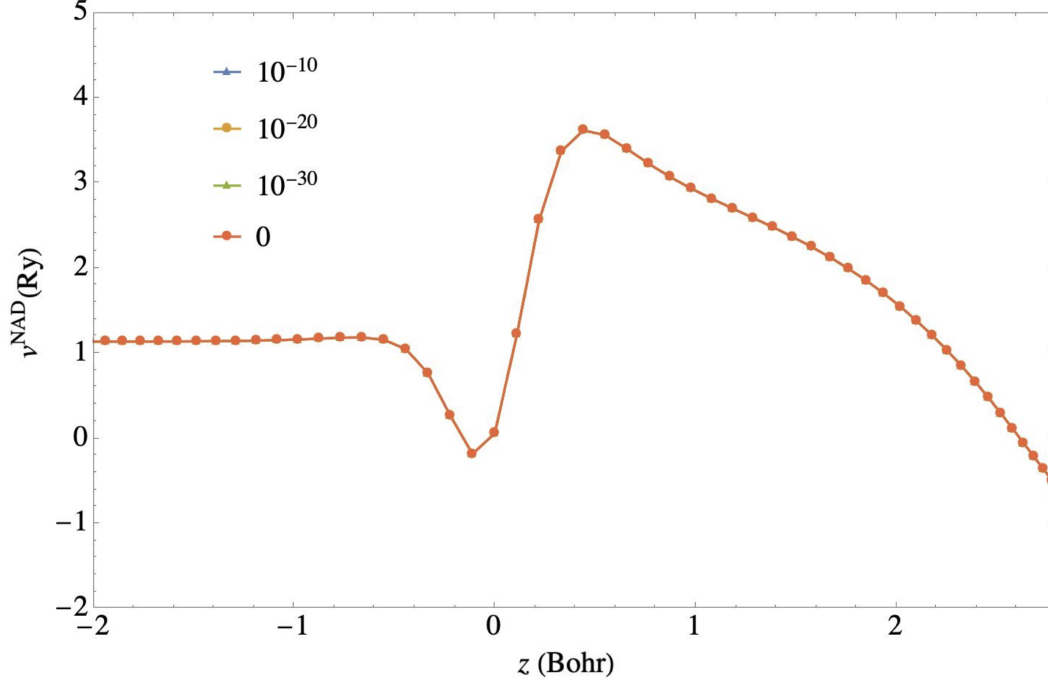

Figure S9: Comparison of  $v^{\text{NAD/INV}}$  with and without  $\delta$  term (in  $\sqrt{e/\text{Bohr}}$ ) added to denominators to avoid singularities. There is no perceptible difference for  $\delta = 0$  and several small values, in this the overlap region of the densities which is our main part of interest, showing that use of  $\delta$  is unnecessary.

## 4 Parameter $\alpha$ in the Fermi-Dirac Distribution Function for Density Localisation

We considered different values of the parameter  $\alpha$  in the Fermi-Dirac distribution function Eq. (26) for density localization from Eq. (27) to ensure meaningful and accurate results. Fig. S10 shows  $v^{\text{NAD/INV}}$  for several values. The shapes are similar, but we see that larger values of  $\alpha$  give a taller and narrower plateau, and a higher barrier. The extreme value of  $100 \text{ Bohr}^{-1}$  also causes discontinuities in the overlap region due to numerical difficulties from the sharp variation of the density  $\rho_B$ , making this value unsuitable (at least given the grid spacing used here). Very small  $\alpha$  such as  $5 \text{ Bohr}^{-1}$  are well behaved, but involve a large overlap between the densities and do not constitute really a partition between the atoms,

so are not of interest for our study here. For calculations in the main text, we choose an intermediate value of  $\alpha = 20 \text{ Bohr}^{-1}$  for  $F(z)$  defined in Eq. (26).

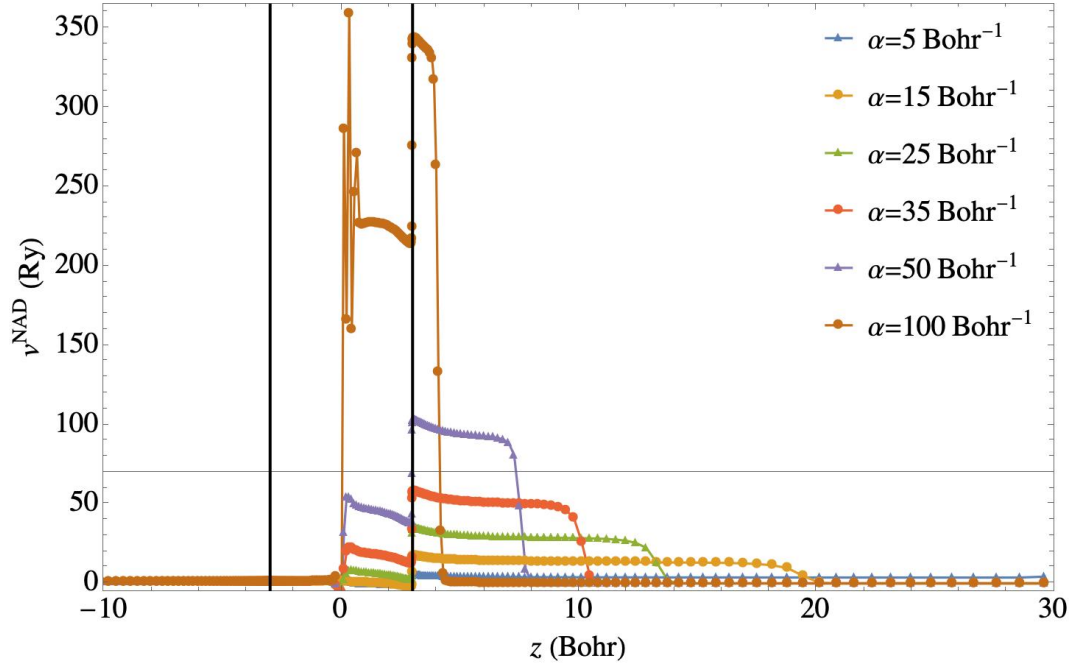

Figure S10: Effect on  $v^{\text{NAD/INV}}$  of changing  $\alpha$  in the function  $F(z)$ . Vertical black lines indicate the  $z$  coordinates of the nuclei at  $\pm 3 \text{ Bohr}$ .

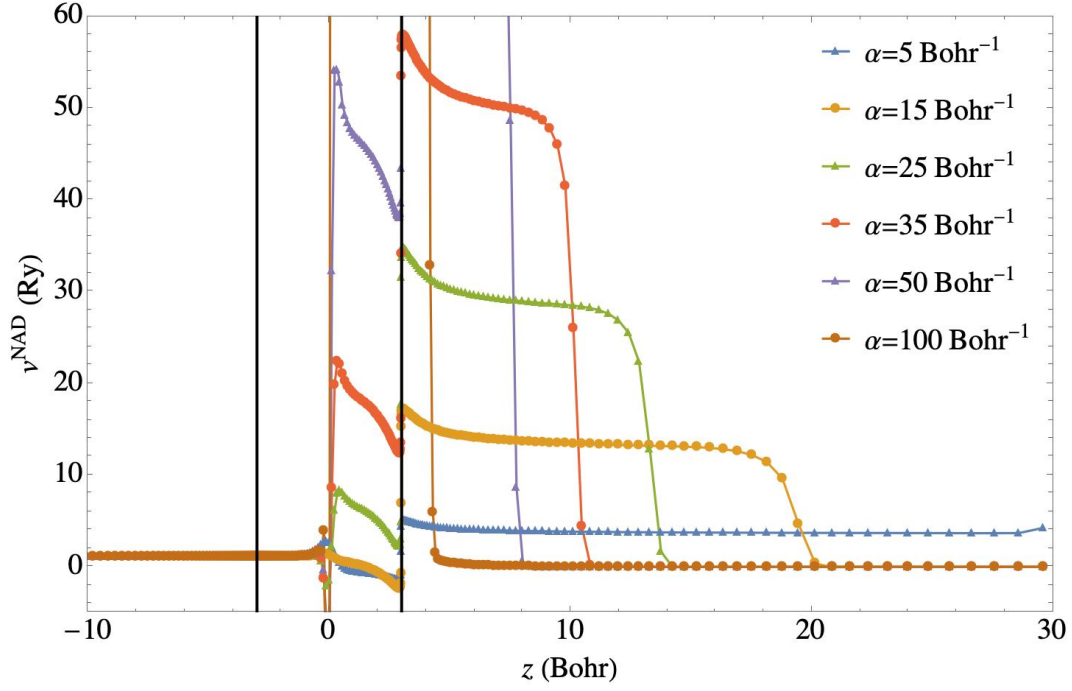

Figure S11: Effect on  $v^{\text{NAD/INV}}$  of changing  $\alpha$  in the function  $F(z)$  with detail on lower heights.

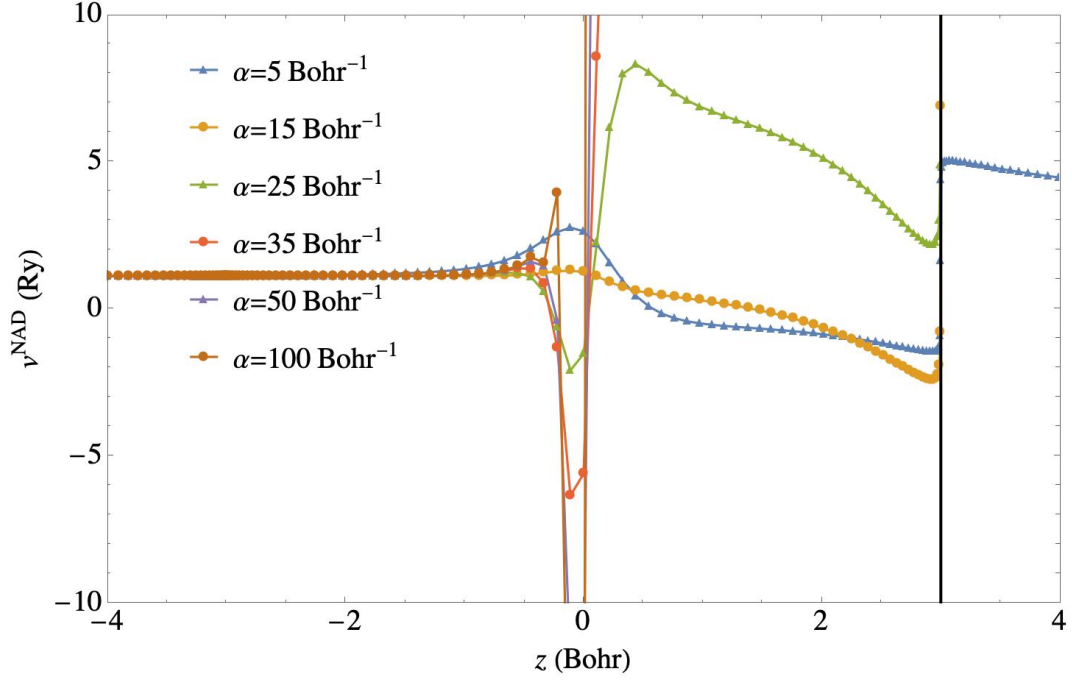

Figure S12: Effect on  $v^{\text{NAD/INV}}$  of changing  $\alpha$  in the function  $F(z)$  with detail in the overlap region.
